# Supplementary material for: Treeging
Source: arXiv:2110.01053 ancillary file (2021-10-03)
Supplement: Supplementary file 2 [file Treeging_Appendix.pdf]

# Treering: Appendix

Gregory L. Watson<sup>1\*</sup>, Michael Jerrett<sup>2</sup>, Colleen E. Reid<sup>3</sup> and Donatello Telesca<sup>1</sup>

<sup>1</sup> Department of Biostatistics, University of California, Los Angeles

<sup>2</sup> Department of Environmental Health Sciences, University of California, Los Angeles

<sup>3</sup> Geography Department, University of Colorado Boulder

October 3, 2021

## A.1 Spatial Simulations

The three informative and 17 spurious spatial simulation covariates were sampled from a Gaussian process with mean 0 and an independent covariance function. The spatial field,  $Y(d)$ , was sampled from a GP with a mean function  $\mu_Y(d)$  depending on three covariates:

$$\mu_Y(d) = \eta * \{X_1(d) + 1[X_2(d) \geq 0] - 1[X_2(d) < 0] + 3[1 + \exp(-2X_3(d) + 3)]^{-1}\}, \quad (1)$$

where  $a$  is the covariate effect size multiplier that scales up or down the strength of the covariate effects. An isotropic exponential covariance function was employed,  $\Sigma(d_1, d_2) = \exp(-\|d_1 - d_2\|/\nu)$ , where  $\nu$  is a parameter determines the strength of spatial dependence for points on the random field that are a distance of  $\|d_1 - d_2\|$  apart.

The values of  $\eta$  and  $\nu$  were varied to investigate model performance under a variety of circumstances. The values of the effect size multiplier,  $\eta$ , were  $\{0, 0.1, 0.2, \dots, 2\}$ , and  $\nu$  varied from zero to 1.25, taking the following values,  $\{0, 0.05, 0.1, 0.125, 0.15, 0.175, 0.2, 0.225, 0.25, 0.275, 0.3, 0.325, 0.35, 0.375, 0.4, 0.425, 0.45, 0.475, 0.5, 0.525, 0.55, 0.575, 0.6, 0.625, 0.65, 0.675, 0.7, 0.725, 0.75, 0.775, 0.8, 0.825, 0.85, 0.875, 0.9, 0.925, 0.95, 0.975, 1, 1.025, 1.05, 1.075, 1.1, 1.125, 1.15, 1.175, 1.2, 1.225, 1.25\}$ .

---

\*gwatson@ucla.edu

The unobserved grid of spatial locations at which  $Y(d)$  was simulated was the cartesian product of 21 evenly spaced points beginning at 0 and ending at 10. The observed data were simulated at 100 locations randomly selected with uniform probability  $\{(s_1, s_2) : s_1, s_2 \in (0, 10)\}$ .

## A.2 Case Study Covariates

| Covariate                                                            | Data Source                           |
|----------------------------------------------------------------------|---------------------------------------|
| Monitor Latitude                                                     | U. S. Environmental Protection Agency |
| Monitor Longitude                                                    | U. S. Environmental Protection Agency |
| Date <sup>1</sup>                                                    | U. S. Environmental Protection Agency |
| Elevation (m)                                                        | National Digital Elevation Model      |
| Boundary Layer Height (m)                                            | Rapid Update Cycle                    |
| Surface Pressure (Pa)                                                | Rapid Update Cycle                    |
| Relative Humidity (%)                                                | Rapid Update Cycle                    |
| Temperature at 2 m (°K)                                              | Rapid Update Cycle                    |
| U-Component of Wind Speed (m/s)                                      | Rapid Update Cycle                    |
| V-Component of Wind Speed (m/s)                                      | Rapid Update Cycle                    |
| Inverse Distance to Nearest Wildfire (m <sup>-1</sup> ) <sup>2</sup> | Fire Inventory from NCAR v1.5         |
| Annual Average Traffic within 1 km                                   | Dynamap 2000, TeleAtlas               |
| Agricultural Land Use within 1 km (%)                                | 2006 National Land Cover Database     |
| Urban Land Use within 1 km (%)                                       | 2006 National Land Cover Database     |
| Vegetation Land Use within 1 km (%)                                  | 2006 National Land Cover Database     |
| Normalized Difference Vegetation Index                               | Landsat Data                          |
| Nitrogen Dioxide (log molecules/cm <sup>2</sup> )                    | Ozone Monitoring Instrument Satellite |
| WRF-Chem PM <sub>2.5</sub> (log kg/day) <sup>3</sup>                 | WRF-Chem                              |
| WRF-Chem Ozone (log 8 Hour Maximum) <sup>4</sup>                     | WRF-Chem                              |

<sup>1</sup> Date was included for space-time simulations only.

<sup>2</sup> Proximity to wildfires was incorporated as inverse distance to the nearest wildfire. See Watson et al. (2019) for details.

<sup>3</sup> Only included as covariate for PM<sub>2.5</sub> case studies.

<sup>4</sup> Only included as covariate for ozone case studies.

### A.3 Spherical Covariance Estimation

The default covariance estimation procedure for treeding fits a spherical variogram to the empirical variogram of the spatial or temporal residuals. For space-time treeding, we assume separability and separately fit spatial and temporal spherical covariances, multiplying them together to estimate the space-time covariance. The residuals are the difference between the fitted and observed training outcomes, i.e.,

$$\mathbf{e}(\mathbf{d}) = \mathbf{y}(\mathbf{d}) - \hat{\mathbf{y}}(\mathbf{d}), \quad (2)$$

where  $\hat{\mathbf{y}}(\mathbf{d}) = T(\mathbf{X}(\mathbf{d}), \boldsymbol{\theta})$  for treeding and  $\hat{\mathbf{y}}(\mathbf{d}) = \mathbf{X}(\mathbf{d})\boldsymbol{\beta}$  for kriging. The empirical variogram is

$$\hat{\gamma}(h \pm \delta) = \frac{1}{2|N(h \pm \delta)|} \sum_{|d_i - d_j| \leq \delta} |y(d_i) - y(d_j)|^2, \quad (3)$$

and the spherical variogram is

$$\gamma(h, r, s, a) = \begin{cases} 0 & h = 0 \\ a + (s - a) \left( \frac{3h}{2r} - \frac{h^3}{2r^3} \right) & 0 < h \leq r \\ s & h > r, \end{cases} \quad (4)$$

and spherical covariance function is

$$C(h, r, s, a) = \begin{cases} s & h = 0 \\ (s - a) \left( 1 - \frac{3h}{2r} + \frac{h^3}{2r^3} \right) & 0 < h \leq r \\ 0 & h > r. \end{cases} \quad (5)$$

### A.4 Space-Time Simulations

Covariates for the space-time simulations were generated from a Gaussian process (GP) with mean 0 and a separable covariance function  $\Sigma_X(d) = \Sigma_X(s)\Sigma_X(t)$ , where  $d = (s, t)$ . Exponential covariance functions with randomly selected range parameters were used for  $\Sigma_X(s)$  and  $\Sigma_X(t)$ . The random field mean  $\mu_Y[\mathbf{X}(d)]$  was a nonlinear function of the first 3 covariates,

$$\mu_Y[\mathbf{X}(d)] = \eta \left\{ \frac{1}{2} X_1(d) + \frac{3}{4} [X_2(d) \leq 0.1] - \frac{3}{4} [X_2(d) > 0.1] + 2 \{1 + \exp[-2X_3(d)]\}^{-1} + X_i(d)X_j(d) \right\}, \quad (6)$$

where  $\eta$  is the covariate effect size multiplier that can be scaled up or down to simulate stronger or weaker covariate effects, and  $i$  and  $j$  are 2 of the 3 informative covariates selected at random. Values of the effect size multiplier  $\eta$  were  $\{0, 0.2, 0.4, \dots, 2\}$ . The additional covariates were included as spurious covariates in scenarios  $B$  and  $D$  to assess the robustness of prediction models.

A separable covariance function was used for  $Y(d)$  with independent exponential spatial and temporal covariance functions. The ranges were varied across the following ranges to investigate the effects of varying levels of spatial and temporal dependence. Values for the spatial covariance range were  $2 - \sqrt{u}$  for  $u \in \{0, 0.25, 0.5, \dots, 4\}$ . Values for the temporal covariance range were  $\{0, 2.5, 5, 7.5, 10\}$ .

The unobserved grid of spatial locations at which  $Y(d)$  was simulated was the cartesian product of 11 evenly spaced points beginning at 0 and ending at 10. The observed data were simulated at 40 spatial locations randomly selected with uniform probability  $\{(s_1, s_2) : s_1, s_2 \in (0, 10)\}$ . Both the observed and unobserved data were simulated over 30 consecutive timepoints, yielding a total of 1,200 observed data points and 3,630.

## References

Watson, G. L., Telesca, D., Reid, C. E., Pfister, G. G., and Jerrett, M. (2019). Machine learning models accurately predict ozone exposure during wildfire events. *Environmental Pollution*, 254:112792.
